# Supplementary material for: Deep Model Merging: The Sister of Neural Network Interpretability -- A Survey
Source: arXiv:2410.12927 source file (2025-03-21)
Supplement: Supplementary file 1 [file 99_appendix.tex]

\section{}
